# Supplementary material for: Updated model-independent measurement of the strong-phase differences between $D^0$ and $\bar{D}^0 \to K^{0}_{S/L}\pi^+\pi^-$ decays
Source: arXiv:2503.22126 source file (2025-04-18)
Supplement: Supplementary file 1 [file corr2.tex]

80&74&22&$-$28&14&62&79&9&28&42&29&16&$-$20&$-$46&$-$46&76&67&69&5&$-$32&$-$1&56&69&$-$7&38&46&27&9&$-$20&$-$44&$-$48\\
$c_{2}$& &71&23&$-$18&19&61&72&4&31&39&29&11&$-$15&$-$41&$-$38&55&87&63&11&$-$22&6&52&60&$-$2&39&43&27&4&$-$15&$-$39&$-$40\\
$c_{3}$& & &47&9&49&80&76&8&24&34&24&$-$4&$-$25&$-$31&$-$25&42&51&86&35&2&31&60&54&$-$1&40&43&20&$-$14&$-$25&$-$31&$-$35\\
$c_{4}$& & & &66&68&47&33&1&$-$30&$-$46&$-$60&$-$16&36&26&12&$-$7&5&27&88&61&60&29&8&$-$23&$-$23&$-$40&$-$63&$-$22&36&27&4\\
$c_{5}$& & & & &61&15&$-$8&4&$-$37&$-$55&$-$54&$-$31&34&46&39&$-$53&$-$30&$-$7&70&98&64&2&$-$31&$-$10&$-$36&$-$51&$-$58&$-$33&34&47&36\\
$c_{6}$& & & & & &52&30&3&$-$11&$-$21&$-$25&$-$23&16&20&22&$-$16&0&28&65&56&90&28&2&$-$2&0&$-$13&$-$30&$-$30&17&20&14\\
$c_{7}$& & & & & & &66&2&13&25&15&$-$14&$-$22&$-$31&$-$14&35&42&62&37&7&34&77&44&$-$5&32&34&12&$-$25&$-$21&$-$32&$-$28\\
$c_{8}$& & & & & & & &11&22&32&20&7&$-$15&$-$33&$-$38&53&58&65&18&$-$14&13&51&83&$-$5&34&39&17&$-$2&$-$15&$-$32&$-$50\\
$s_{1}$& & & & & & & & &17&5&0&19&6&11&6&2&10&13&$-$3&5&5&1&7&17&9&5&$-$1&19&7&12&1\\
$s_{2}$& & & & & & & & & &50&49&19&$-$40&$-$29&$-$15&26&24&31&$-$32&$-$37&$-$14&11&23&21&78&51&49&17&$-$40&$-$29&$-$17\\
$s_{3}$& & & & & & & & & & &84&$-$9&$-$73&$-$58&$-$39&46&43&47&$-$38&$-$55&$-$20&33&42&10&54&98&84&$-$11&$-$73&$-$57&$-$41\\
$s_{4}$& & & & & & & & & & & &$-$7&$-$73&$-$55&$-$29&36&36&37&$-$47&$-$53&$-$23&23&31&12&52&82&99&$-$8&$-$73&$-$54&$-$32\\
$s_{5}$& & & & & & & & & & & & &35&11&8&14&9&$-$8&$-$41&$-$34&$-$40&$-$26&2&37&23&$-$6&$-$3&83&35&9&8\\
$s_{6}$& & & & & & & & & & & & & &54&35&$-$29&$-$19&$-$38&18&33&9&$-$33&$-$28&13&$-$43&$-$70&$-$72&36&98&54&42\\
$s_{7}$& & & & & & & & & & & & & & &56&$-$51&$-$45&$-$44&19&46&17&$-$49&$-$48&27&$-$30&$-$55&$-$55&12&55&95&60\\
$s_{8}$& & & & & & & & & & & & & & & &$-$49&$-$42&$-$42&4&36&14&$-$36&$-$57&39&$-$9&$-$33&$-$28&6&36&52&85\\
$c'_{2}$& & & & & & & & & & & & & & & & &64&56&$-$11&$-$56&$-$19&46&69&$-$17&30&46&36&11&$-$30&$-$50&$-$49\\
$c'_{3}$& & & & & & & & & & & & & & & & & &59&3&$-$32&$-$2&48&62&$-$9&25&44&35&6&$-$20&$-$43&$-$41\\
$c'_{4}$& & & & & & & & & & & & & & & & & & &31&$-$9&26&65&63&$-$14&35&48&33&$-$13&$-$38&$-$41&$-$47\\
$c'_{5}$& & & & & & & & & & & & & & & & & & & &69&72&34&5&$-$42&$-$33&$-$37&$-$52&$-$43&18&21&$-$0\\
$c'_{6}$& & & & & & & & & & & & & & & & & & & & &63&$-$0&$-$33&$-$14&$-$42&$-$54&$-$57&$-$34&34&48&36\\
$c'_{7}$& & & & & & & & & & & & & & & & & & & & & &30&$-$0&$-$19&$-$16&$-$18&$-$28&$-$42&9&19&11\\
$c'_{8}$& & & & & & & & & & & & & & & & & & & & & & &50&$-$26&16&33&20&$-$30&$-$33&$-$47&$-$41\\
$c'_{9}$& & & & & & & & & & & & & & & & & & & & & & & &$-$16&26&43&30&$-$1&$-$29&$-$46&$-$65\\
$s'_{1}$& & & & & & & & & & & & & & & & & & & & & & & & &32&16&14&34&14&24&44\\
$s'_{2}$& & & & & & & & & & & & & & & & & & & & & & & & & &60&51&16&$-$42&$-$32&$-$17\\
$s'_{3}$& & & & & & & & & & & & & & & & & & & & & & & & & & &82&$-$10&$-$70&$-$55&$-$38\\
$s'_{4}$& & & & & & & & & & & & & & & & & & & & & & & & & & & &$-$4&$-$71&$-$55&$-$31\\
$s'_{5}$& & & & & & & & & & & & & & & & & & & & & & & & & & & & &35&11&10\\
$s'_{6}$& & & & & & & & & & & & & & & & & & & & & & & & & & & & & &54&43\\
$s'_{7}$& & & & & & & & & & & & & & & & & & & & & & & & & & & & & & &58\\
